# Supplementary material for: Fluctuations superconductivity and giant negative magnetoresistance in a gate voltage tuned 2D electron liquid with strong spin-orbit impurity scattering
Source: arXiv:2006.05098 ancillary file (2021-03-29)
Supplement: Supplementary file 1 [file PRLSMRev.pdf]

# Fluctuations superconductivity and giant negative magnetoresistance in a gate voltage tuned 2D electron liquid with strong spin-orbit impurity scattering

## I. DETAILS OF THE MODEL AND FORMULATION

We assume, for simplicity of the analysis, that impurity scatterings are dominated by the spin-orbit interaction. We use a reference of frame in which the conducting interface is in its  $z-x$  plane, with the in-plane electric and magnetic fields:  $\mathbf{E}=\hat{x}E$ ,  $\mathbf{B}=\hat{z}H$ , respectively. The electrons are confined within a thin rectangular film of thickness  $d$  along the  $y$  axis. Linear response is assumed with respect to the electric field. To take into account the orbital magnetic field effect one should invoke gauge invariance in evaluating the Cooper-pair fluctuations kinetic energy  $(1/2)Dq^2$ . Since the film thickness  $d$  is much smaller than the Cooper-pair coherence length, this can be done approximately by replacing  $q^2$  with:  $q_y^2 + \langle (q_x + \frac{2e}{\hbar c}Hy)^2 \rangle = q^2 + (\frac{2e}{\hbar c}H)^2 \langle y^2 \rangle + 2q_x \frac{2e}{\hbar c}H \langle y \rangle = q^2 + 2(edH/\hbar)^2$ , where the average is over the narrow film dimension.

In this section we avoid the complexity of the LAO/STO (111) interface band structure by assuming a single-band 2D electron-gas model with an effective DOS function  $N_{2D} = m^*/2\pi\hbar^2$ . The underlying spin-orbit induced band mixing will be considered in the next section, within a minimal model of piecewise DOS function  $N_{2D}(E)$ , when interaction between fluctuations will be considered.

Starting with the Nambu field operators:

$$\Psi(\mathbf{r}; \tau) \equiv \begin{bmatrix} \psi_{\uparrow}(\mathbf{r}; \tau) \\ \psi_{\downarrow}(\mathbf{r}; \tau) \\ \psi_{\uparrow}^{\dagger}(\mathbf{r}; \tau) \\ \psi_{\downarrow}^{\dagger}(\mathbf{r}; \tau) \end{bmatrix}, \quad (1)$$

$$\Psi^{\dagger}(\mathbf{r}; t) \equiv \begin{bmatrix} \psi_{\uparrow}^{\dagger}(\mathbf{r}; \tau) & \psi_{\downarrow}^{\dagger}(\mathbf{r}; \tau) & \psi_{\uparrow}(\mathbf{r}; \tau) & \psi_{\downarrow}(\mathbf{r}; \tau) \end{bmatrix}$$

the Nambu-Gor'kov time-ordered Green's functions  $4 \times 4$  matrix is defined by:

$$\mathcal{G}(\mathbf{r}, \mathbf{r}'; \tau, \tau') \equiv -\langle T_{\tau} \Psi(\mathbf{r}; \tau) \Psi^{\dagger}(\mathbf{r}'; \tau') \rangle \quad (2)$$

$$\equiv \begin{pmatrix} \mathcal{G}_{11}(\mathbf{r}, \mathbf{r}'; \tau, \tau') & \mathcal{G}_{12}(\mathbf{r}, \mathbf{r}'; \tau, \tau') \\ \mathcal{G}_{21}(\mathbf{r}, \mathbf{r}'; \tau, \tau') & \mathcal{G}_{22}(\mathbf{r}, \mathbf{r}'; \tau, \tau') \end{pmatrix}$$

where  $T_{\tau}$  is the time ordered operator and  $\tau, \tau'$  are imaginary (Matzubara) time variables.

The  $2 \times 2$  Green's functions and anomalous Green's functions sub-matrices relevant to our problem are:

$$\mathcal{G}_{11}(\mathbf{r}, \mathbf{r}'; \tau, \tau') = -\left\langle T_{\tau} \begin{pmatrix} \psi_{\uparrow}(\mathbf{r}; \tau) \psi_{\uparrow}^{\dagger}(\mathbf{r}'; \tau') & \psi_{\uparrow}(\mathbf{r}; \tau) \psi_{\downarrow}^{\dagger}(\mathbf{r}'; \tau') \\ \psi_{\downarrow}(\mathbf{r}; \tau) \psi_{\uparrow}^{\dagger}(\mathbf{r}'; \tau') & \psi_{\downarrow}(\mathbf{r}; \tau) \psi_{\downarrow}^{\dagger}(\mathbf{r}'; \tau') \end{pmatrix} \right\rangle,$$

$$\mathcal{G}_{21}(\mathbf{r}, \mathbf{r}'; \tau, \tau') = -\left\langle T_{\tau} \begin{pmatrix} \psi_{\uparrow}^{\dagger}(\mathbf{r}; \tau) \psi_{\uparrow}^{\dagger}(\mathbf{r}'; \tau') & \psi_{\uparrow}^{\dagger}(\mathbf{r}; \tau) \psi_{\downarrow}^{\dagger}(\mathbf{r}'; \tau') \\ \psi_{\downarrow}^{\dagger}(\mathbf{r}; \tau) \psi_{\uparrow}^{\dagger}(\mathbf{r}'; \tau') & \psi_{\downarrow}^{\dagger}(\mathbf{r}; \tau) \psi_{\downarrow}^{\dagger}(\mathbf{r}'; \tau') \end{pmatrix} \right\rangle$$

In terms of these Green's functions we write the reduced subset of Gor'kov's equations in real space, describing s-wave spin-singlet pairing, as:

$$\left[ (\hbar\partial_{\tau} - \hat{\xi}) \sigma_0 - \sigma_z \mu_B H \right] \mathcal{G}_{11}(\mathbf{r}, \mathbf{r}'; \tau, \tau') - \int d^2 r'' \mathcal{V}(\mathbf{r}, \mathbf{r}'') \mathcal{G}_{11}(\mathbf{r}'', \mathbf{r}'; \tau, \tau') \\ - i\sigma_y \Delta(\mathbf{r}, \tau) \mathcal{G}_{21}(\mathbf{r}, \mathbf{r}'; \tau, \tau') = \sigma_0 \delta(\tau - \tau') \delta(\mathbf{r} - \mathbf{r}') \quad (3)$$

$$i\sigma_y \Delta^*(\mathbf{r}, \tau) \mathcal{G}_{11}(\mathbf{r}, \mathbf{r}'; \tau, \tau') + \left[ (\hbar\partial_{\tau} + \hat{\xi}) \sigma_0 + \sigma_z \mu_B H \right] \mathcal{G}_{21}(\mathbf{r}, \mathbf{r}'; \tau, \tau') \\ + \int d^2 r'' \mathcal{V}(\mathbf{r}, \mathbf{r}'') \mathcal{G}_{21}(\mathbf{r}'', \mathbf{r}'; \tau, \tau') = 0 \quad (4)$$

where  $\mu_B = e\hbar/2m_e$  is the Bohr magneton,  $\sigma_0, \sigma_y, \sigma_z$ , are the  $2 \times 2$  unity, and the  $y, z$  Pauli matrices, respectively, and  $\Delta_{\downarrow\uparrow}(\mathbf{r}, \tau) = -\Delta_{\uparrow\downarrow}(\mathbf{r}, \tau) \equiv \Delta(\mathbf{r}, \tau)$ —the components of the order-parameter matrix responsible for spin-singlet pairing. In these equations the impurity-scattering matrix is given by [1],[2]:

$$\mathcal{V}(\mathbf{r}, \mathbf{r}') = \frac{1}{d} \sum_n \int \frac{d^2 p}{(2\pi)^2} \int \frac{d^2 q}{(2\pi)^2} \times \exp \left\{ i\mathbf{p} \cdot \left[ \frac{1}{2} (\mathbf{r} + \mathbf{r}') - \mathbf{R}_n \right] + i\mathbf{q} \cdot (\mathbf{r} - \mathbf{r}') \right\} (iV_{SO} [\hat{\mathbf{p}} \times \hat{\mathbf{q}}] \cdot \sigma) \quad (5)$$

where  $\mathbf{R}_n$  is a position vector of an impurity and  $[\hat{\mathbf{p}} \times \hat{\mathbf{q}}] \cdot \sigma = \pm |\hat{\mathbf{p}} \times \hat{\mathbf{q}}| \sigma_y$ , depending on whether  $[\hat{\mathbf{p}} \times \hat{\mathbf{q}}]$  is oriented parallel (+) or antiparallel (−) to the  $y$  axis. The strong spin-orbit interaction of the Ti 3d conduction electrons with lattice ions in SrTiO<sub>3</sub> [3] motivates our use of Eq.5 as the spin-orbit impurity scattering matrix of free electrons in the LAO/STO (111) interface.

The temporal Fourier transform, with the fermionic Matsubara frequency,  $\omega_n = (2n+1)\pi k_B T/\hbar$ , of the integral equation for the normal state Green's functions matrix  $\tilde{\mathcal{G}}_{11}^{(0)}(\mathbf{r}, \mathbf{r}'; \omega_n)$  in the presence of the spin-orbital impurity scattering, obtained from Eq.3 with  $\Delta(\mathbf{r}, \tau) = 0$ , is written as:

$$\tilde{\mathcal{G}}_{11}^{(0)}(\mathbf{r}, \mathbf{r}'; \omega_n) = \mathcal{G}_{11}^{(0)}(\mathbf{r}, \mathbf{r}'; \omega_n) + \int d^2 r_1 \int d^2 r_2 \mathcal{G}_{11}^{(0)}(\mathbf{r}, \mathbf{r}_1; \omega_n) \mathcal{V}(\mathbf{r}_1, \mathbf{r}_2) \tilde{\mathcal{G}}_{11}^{(0)}(\mathbf{r}_2, \mathbf{r}'; \omega_n) \quad (6)$$

where:

$$\left[ (i\hbar\omega_n - \hat{\xi}) \sigma_0 - \sigma_z \mu_B H \right] \mathcal{G}_{11}^{(0)}(\mathbf{r}, \mathbf{r}'; \omega_n) = \sigma_0 \delta(\mathbf{r} - \mathbf{r}') \quad (7)$$

In attempting to find the desired linear TDGL equation, we focus our attention on the pairing self-consistency equation, to first order in the pair-potential expansion. In terms of the Nambu  $2 \times 2$  anomalous Green's functions matrix, this equation takes the form:

$$Tr \left\langle i\sigma_y \tilde{\mathcal{G}}_{21}^{(1)}(\mathbf{r}, \mathbf{r}; \tau, \tau) \right\rangle_{imp} g = \Delta^*(\mathbf{r}, \tau) \quad (8)$$

where

$$\left\langle \tilde{\mathcal{G}}_{21}^{(1)}(\mathbf{r}, \mathbf{r}; \tau, \tau) \right\rangle_{imp} = \int d^2 r'' \int_0^\beta d\tau'' \left\langle \tilde{\mathcal{G}}_{11}^{(0)T}(\mathbf{r}, \mathbf{r}''; \tau'' - \tau) i\sigma_y \tilde{\mathcal{G}}_{11}^{(0)}(\mathbf{r}, \mathbf{r}''; \tau'' - \tau) \right\rangle_{imp} \Delta^*(\mathbf{r}'', \tau'')$$

and  $g < 0$  is the BCS coupling constant, and the average is over impurity positions.

Fourier transforming, both spatially and temporally, with wavevector  $\mathbf{q}$  and bosonic Matsubara frequency  $\Omega_\nu = 2\nu\pi k_B T/\hbar \geq 0$ , respectively, the self-consistency equation reads:

$$\begin{aligned} & \int d^2 r e^{-i\mathbf{q} \cdot \mathbf{r}} \int_0^\beta d\tau e^{i\Omega_\nu \tau} Tr \left\langle i\sigma_y \tilde{\mathcal{G}}_{21}^{(1)}(\mathbf{r}, \mathbf{r}; \tau, \tau) \right\rangle_{imp} \\ & \equiv N_{2D} k_B T \sum_{n=-\infty}^{\infty} Tr \left[ i\sigma_y \tilde{\mathcal{S}}(\mathbf{q}; \omega_n, -\omega_n + \Omega_\nu) \right] \Delta^*(\mathbf{q}, \Omega_\nu) = \Delta^*(\mathbf{q}, \Omega_\nu) / g, \end{aligned} \quad (9)$$

$$\tilde{\mathcal{S}}(\mathbf{q}; \omega_n, -\omega_n + \Omega_\nu) = \begin{pmatrix} 0 & \tilde{S}_{\uparrow\downarrow}(\mathbf{q}; \omega_n, -\omega_n + \Omega_\nu) \\ \tilde{S}_{\downarrow\uparrow}(\mathbf{q}; \omega_n, -\omega_n + \Omega_\nu) & 0 \end{pmatrix} \quad (10)$$

where  $N_{2D} = m^*/2\pi\hbar^2$  is the single electron density of states, per unit area, per spin, and the kernel  $\tilde{\mathcal{S}}(\mathbf{q}; \omega_n, -\omega_n + \Omega_\nu)$  (see Ref.[4]) plays the role of vertex of the pair-potential, "dressed" by the impurity scattering effect. It is calculated by exploiting the standard ladder diagrams expansion for the vertex part [5], consistently with the corresponding non-crossing diagrams contributing to the self-energy [2].

Thus, in terms of the components of  $\tilde{\mathcal{S}}(\mathbf{q}; \omega_n, -\omega_n + \Omega_\nu)$  (see Eq.10) Eq.8 reads (after changing  $n \rightarrow -n$  under the frequency summation):

$$\begin{aligned} & k_B T \sum_{n=-\infty}^{\infty} \left[ \tilde{S}_{\downarrow\uparrow}(\mathbf{q}; -\omega_n, \omega_n + \Omega_\nu) - \tilde{S}_{\uparrow\downarrow}(\mathbf{q}; -\omega_n, \omega_n + \Omega_\nu) \right] \\ & = 2k_B T \sum_{n=-\infty}^{\infty} \tilde{S}_{\downarrow\uparrow}(\mathbf{q}; -\omega_n, \omega_n + \Omega_\nu) = 1/|g| N_{2D} \end{aligned} \quad (11)$$

Note that the second equality in Eq.11 is implied by the property:  $\tilde{S}_{\downarrow\downarrow}(\mathbf{q}; \omega_n, -\omega_n + \Omega_\nu) = -\tilde{S}_{\downarrow\uparrow}(\mathbf{q}; -\omega_n + \Omega_\nu, \omega_n)$ . The calculation of the kernel  $\tilde{S}_{\downarrow\uparrow}(\mathbf{q}; -\omega_n + \Omega_\nu, \omega_n)$  is carried out in two steps. In the first step, we neglect vertex corrections, but insert self energy into the Matzubara frequencies,  $\omega_n \rightarrow \tilde{\omega}_n = \omega_n + (1/2\tau_{SO}) \text{sgn}(\omega_n)$ , where:  $1/\tau_{SO} \equiv n_i N_{2D}(0) \int_0^{2\pi} d\theta \sin^2 \theta V_{SO}^2(\theta) = \pi N_{2D} n_i V_{SO}^2$ , with  $n_i$  standing for the density of impurities per unit area, and find that:

$$S_{\downarrow\downarrow}^0(\mathbf{q}; -\omega_n, \omega_n + \Omega_\nu) \simeq \frac{2\pi\theta(\omega_{n+\nu}\omega_n) \text{sign}(\omega_{n+\nu} + \omega_n)}{\hbar(\tilde{\omega}_{n+\nu} + \tilde{\omega}_n) - 2i\mu_B H} \left[ 1 - \frac{1}{2} \left( \frac{v_F}{\tilde{\omega}_{n+\nu} + \tilde{\omega}_n - 2i\mu_B H/\hbar} \right)^2 q^2 \right] \\ \equiv S_-^0(\omega_n; q, \Omega_\nu), \quad (12)$$

$$S_{\downarrow\uparrow}^0(\mathbf{q}; -\omega_n, \omega_n + \Omega_\nu) \simeq \frac{2\pi\theta(\omega_{n+\nu}\omega_n) \text{sign}(\omega_{n+\nu} + \omega_n)}{\hbar(\tilde{\omega}_{n+\nu} + \tilde{\omega}_n) + 2i\mu_B H} \left[ 1 - \frac{1}{2} \left( \frac{v_F}{\tilde{\omega}_{n+\nu} + \tilde{\omega}_n + 2i\mu_B H/\hbar} \right)^2 q^2 \right] \\ \equiv S_+^0(\omega_n; q, \Omega_\nu) \quad (13)$$

Here expansion has been made, up to second order in the small wavenumber  $q$ . These expressions can be simplified by exploiting the dirty limit of the impurity scattering in the pre-factors of  $q^2$ , i.e. by assuming  $\hbar/\tau_{SO} \gg 2\pi k_B T, 2\mu_B H$ , and approximating  $v_F^2/(\tilde{\omega}_{n+\nu} + \tilde{\omega}_n \pm 2i\mu_B H/\hbar)^2 \approx \tau_{SO}^2 v_F^2$ , so that:

$$S_{\pm}^0(\omega_n; q, \Omega_\nu) \approx \frac{\pi}{\hbar} \frac{\theta(\omega_{n+\nu}\omega_n) (1 - \frac{1}{2}\tau_{SO}^2 v_F^2 q^2)}{|\omega_n + \Omega_\nu/2| + 1/2\tau_{SO} \pm iI \text{sign}(\omega_{n+\nu} + \omega_n)} \quad (14)$$

where  $I \equiv \mu_B H/\hbar$ .

In the second step of the calculation of the kernel  $\tilde{S}_{\downarrow\uparrow}(\mathbf{q}; -\omega_n + \Omega_\nu, \omega_n)$  vertex corrections are taken into account by using the ladder approximation [5]. The algebraic coupled equations equivalent to the entire ladder-diagram summations are given by:

$$\tilde{S}_-(\omega_n; q, \Omega_\nu) = S_-^0(\omega_n; q, \Omega_\nu) \left[ 1 + (2\pi\tau_{SO})^{-1} \tilde{S}_+(\omega_n; q, \Omega_\nu) \right], \quad (15)$$

$$\tilde{S}_+(\omega_n; q, \Omega_\nu) = S_+^0(\omega_n; q, \Omega_\nu) \left[ 1 + (2\pi\tau_{SO})^{-1} \tilde{S}_-(\omega_n; q, \Omega_\nu) \right] \quad (16)$$

with:  $\tilde{S}_-(\omega_n; q, \Omega_\nu) \equiv \tilde{S}_{\downarrow\downarrow}(\mathbf{q}; -\omega_n, \omega_n + \Omega_\nu)$ ,  $\tilde{S}_+(\omega_n; q, \Omega_\nu) \equiv \tilde{S}_{\downarrow\uparrow}(\mathbf{q}; -\omega_n, \omega_n + \Omega_\nu)$ .

Solving Eqs.15,16 and using Eq.14, we find:

$$\tilde{S}_{\pm}(\omega_n; q, \Omega_\nu) \approx \left( \frac{\pi}{\hbar} \right) \theta(\omega_{n+\nu}\omega_n) \frac{|\omega_n + \Omega_\nu/2| + a_q + b \mp iI \text{sign}(\omega_n + \Omega_\nu/2)}{(|\omega_n + \Omega_\nu/2| + a_q)^2 - b^2 + I^2} \quad (17)$$

with:  $a_q \equiv b + Dq^2/2$ ,  $b \equiv 1/2\tau_{SO}$ , and  $D \equiv \tau_{SO} v_F^2/2$  -the electronic diffusion coefficient. Eq.17 is consistent with the vertex function derived by Maki in [5].

Note that in our model the relaxation rate  $1/\tau_{SO}$  plays a dual role; on one hand it represents scattering rate of electrons by impurities, and on the other hand it appears as an energy parameter suppressing the pair-breaking effect of the Zeeman spin-splitting. An extended version of this model, in which additional non-magnetic impurity scattering channel is present, was used in the early literature [5],[2]. In the present model, for the sake of simplicity of the analysis, similar to Fulde and Maki [6], we neglect this non-magnetic component since the effect of impurity scattering is essentially well represented by the magnetic component.

Using Eq.17 in Eq.11 by performing the Matzubara frequency-summation the self-consistency equation takes the form:

$$\ln \left( \frac{T}{T_{c0}} \right) + \frac{1}{2} \left\{ \left( 1 + \frac{b}{\sqrt{b^2 - I^2}} \right) \psi(1/2 + \overline{\kappa}_- + x + y) + \left( 1 - \frac{b}{\sqrt{b^2 - I^2}} \right) \psi(1/2 + \overline{\kappa}_+ + x + y) \right\} - \psi(1/2) = 0 \quad (18)$$

where:

$$\overline{\kappa}_{\pm} \equiv \hbar\kappa_{\pm}/2\pi k_B T, \kappa_{\pm} \equiv D(edH/\hbar)^2 + b \pm \sqrt{b^2 - I^2} \geq 0, \quad (19)$$

$$x \equiv \hbar D q^2 / 4\pi k_B T, y \equiv \hbar \Omega_\nu / 4\pi k_B T \quad (20)$$

and  $T_{c0} \simeq 2e\gamma T_D e^{-1/|g|N_{2D}}$ , with  $\gamma \simeq 0.5772$ , is the mean-field transition temperature at zero magnetic field.

Note that in the single-band model employed in the above calculations the presence of the spin-orbit interaction does not influence  $T_{c0}$ , which is given by the simple BCS expression with the DOS function  $N_{2D} = m^*/2\pi\hbar^2$ .

Note also that in Eq.18 the explicit logarithmic singularity at  $T = 0$  is canceled by the asymptotic logarithmic divergence of the digamma function whenever  $\varkappa_+(q, \Omega_\nu) > 0$ , a result equivalent to the removal of the Cooper singularity by finite magnetic field or/and by  $\Omega_\nu > 0$ .

## II. INTERACTION BETWEEN FREE (GAUSSIAN) FLUCTUATIONS

Interactions between free (Gaussian) fluctuations are introduced by taking into account higher-order terms in the pair-potential expansion of Eq.4. The leading-order contribution to the interaction is the cubic term in this expansion obtained by substituting the first order term to Eq.3 and then back to Eq.4. Exploiting the Hartree decoupling amounts to linearization of the cubic term resulting in the following correction to  $\mathcal{G}_{21}$ :

$$\delta\mathcal{G}_{21}^{(3)}(\mathbf{r}, \mathbf{r}'; \tau, \tau') \equiv \mathcal{G}_{21}^{(3)}(\mathbf{r}, \mathbf{r}'; \tau, \tau') - \mathcal{G}_{21}^{(1)}(\mathbf{r}, \mathbf{r}'; \tau, \tau') \quad (21)$$

with:

$$\begin{aligned} \delta\mathcal{G}_{21}^{(3)}(\mathbf{r}, \mathbf{r}'; \tau, \tau') &= \int d^2r'' \int_0^\beta d\tau'' \int d^2r_1 \int_0^\beta d\tau_1 \int d^2r_2 \int_0^\beta d\tau_2 \times \\ &\mathcal{G}_{11}^{(0)T}(\mathbf{r}, \mathbf{r}''; \tau'' - \tau) i\sigma_y^{(0)} \mathcal{G}_{11}^{(0)}(\mathbf{r}_1, \mathbf{r}''; \tau'' - \tau_1) i\sigma_y \mathcal{G}_{11}^{(0)T}(\mathbf{r}_1, \mathbf{r}_2; \tau_2 - \tau_1) i\sigma_y \mathcal{G}_{11}^{(0)}(\mathbf{r}', \mathbf{r}_2; \tau_2 - \tau') \times \\ &[k_B T D(\mathbf{r}'' - \mathbf{r}'; \tau'' - \tau') \Delta^*(\mathbf{r}_2, \tau_2) + k_B T D(\mathbf{r}_2 - \mathbf{r}_1; \tau_2 - \tau_1) \Delta^*(\mathbf{r}'', \tau'')] \end{aligned} \quad (22)$$

where:  $\langle \Delta^*(\mathbf{r}_2, \tau_2) \Delta(\mathbf{r}_1, \tau_1) \rangle = k_B T D(\mathbf{r}_2 - \mathbf{r}_1; \tau_2 - \tau_1) \equiv D_T(\mathbf{r}_2 - \mathbf{r}_1; \tau_2 - \tau_1)$  and  $D(\mathbf{r}_2 - \mathbf{r}_1; \tau_2 - \tau_1)$  is the free (Gaussian) fluctuation propagator, whose spatial-temporal Fourier transform, extracted from Eq.18, is given by:

$$D(q, \Omega_\nu)^{-1} = N_{2D} \left\{ \begin{aligned} &\ln\left(\frac{T}{T_{c0}}\right) + \frac{1}{2} \left(1 + \frac{b}{\sqrt{b^2 - T^2}}\right) \psi(1/2 + \overline{\varkappa}_+ + x + y) \\ &+ \frac{1}{2} \left(1 - \frac{b}{\sqrt{b^2 - T^2}}\right) \psi(1/2 + \overline{\varkappa}_- + x + y) - \psi(1/2) \end{aligned} \right\} \quad (23)$$

The corresponding corrected self-consistency (SC) pairing equation in momentum-energy domain is given by:

$$\int d^2r e^{-i\mathbf{q}\cdot\mathbf{r}} \int_0^\beta d\tau e^{i\Omega_\nu\tau} \left[ \begin{aligned} &Tr \left\langle i\sigma_y \tilde{\mathcal{G}}_{21}^{(1)}(\mathbf{r}, \mathbf{r}; \tau, \tau) \right\rangle_{imp} \\ &+ Tr \left\langle i\sigma_y \delta\mathcal{G}_{21}^{(3)}(\mathbf{r}, \mathbf{r}; \tau, \tau) \right\rangle_{imp} \end{aligned} \right] g = \Delta^*(\mathbf{q}, \Omega_\nu) \quad (24)$$

with the kernel,  $\delta\tilde{\mathcal{S}}^{(3)}$ , of the cubic term defined by:

$$\begin{aligned} &\int d^2r e^{-i\mathbf{q}\cdot\mathbf{r}} \int_0^\beta d\tau e^{i\Omega_\nu\tau} \left\langle \delta\tilde{\mathcal{G}}_{21}^{(3)}(\mathbf{r}, \mathbf{r}; \tau, \tau) \right\rangle_{imp} \\ &\equiv 2\Delta^*(\mathbf{q}, \Omega_\nu) N_{2D} \int \frac{d^2q'}{(2\pi)^2} D_T(q') k_B T \sum_{n=-\infty}^{\infty} \delta\tilde{\mathcal{S}}^{(3)}(\mathbf{q}, \mathbf{q}'; \omega_n, \Omega_\nu - \omega_n) \end{aligned} \quad (25)$$

where  $D_T(q') \equiv k_B T D(q', 0)$ . Now, the crucial importance of the correction term is near the vanishing of the "bare" linear term at the critical point, where  $q = 0$ ,  $\Omega_\nu = 0$ . Thus, exploiting also the critical divergence of  $D_T(q')$  at  $q' = 0$ , the dependence of the electronic kernel  $\delta\tilde{\mathcal{S}}^{(3)}$  on the very small wavevectors  $\mathbf{q}, \mathbf{q}'$  and frequency  $\Omega_\nu$  of the fluctuations can be safely neglected, so that in Eq.25 one may assume that:  $\delta\tilde{\mathcal{S}}^{(3)}(\mathbf{q}, \mathbf{q}'; \omega_n, \Omega_\nu - \omega_n) \approx \delta\tilde{\mathcal{S}}^{(3)}(\mathbf{q} = \mathbf{0}, \mathbf{q}' = \mathbf{0}; \omega_n, -\omega_n) \equiv \delta\tilde{\mathcal{S}}^{(3)}(\omega_n)$  and rewrite it in the form:

$$\int d^2r e^{-i\mathbf{q}\cdot\mathbf{r}} \int_0^\beta d\tau e^{i\Omega_\nu\tau} \left\langle \delta\tilde{\mathcal{G}}_{21}^{(3)}(\mathbf{r}, \mathbf{r}; \tau, \tau) \right\rangle_{imp} \approx 2\Delta^*(\mathbf{q}, \Omega_\nu) \int \frac{d^2q'}{(2\pi)^2} D_T(q') k_B T \sum_{n=-\infty}^{\infty} N_{2D} \delta\tilde{\mathcal{S}}^{(3)}(\omega_n) \quad (26)$$

where the undressed kernel, i.e. prior to inserting the self-energy and vertex corrections, is given by:

$$N_{2D}\delta\mathcal{S}^{(3)}(\omega_n) = \int \frac{d^2p}{(2\pi)^2} \mathcal{G}_{11}^{(0)T}(\mathbf{p}, \omega_n) i\sigma_y \mathcal{G}_{11}^{(0)}(-\mathbf{p}, -\omega_n) i\sigma_y \mathcal{G}_{11}^{(0)T}(\mathbf{p}, \omega_n) i\sigma_y \mathcal{G}_{11}^{(0)}(-\mathbf{p}, -\omega_n)$$

with:

$$\mathcal{G}_{11}^{(0)}(\mathbf{p}, \omega_n) = \begin{pmatrix} G_-^{(0)}(\mathbf{p}, \omega_n) & 0 \\ 0 & G_+^{(0)}(\mathbf{p}, \omega_n) \end{pmatrix} = \begin{pmatrix} (i\hbar\omega_n - \xi_p - \mu_B H)^{-1} & 0 \\ 0 & (i\hbar\omega_n - \xi_p + \mu_B H)^{-1} \end{pmatrix}$$

$$\delta\mathcal{S}^{(3)}(\omega_n) = \begin{pmatrix} 0 & \delta\mathcal{S}_{\uparrow\downarrow}^{(3)}(\omega_n) \\ \delta\mathcal{S}_{\downarrow\uparrow}^{(3)}(\omega_n) & 0 \end{pmatrix} \equiv \begin{pmatrix} 0 & \delta\mathcal{S}_-^{(3)}(\omega_n) \\ \delta\mathcal{S}_+^{(3)}(\omega_n) & 0 \end{pmatrix}$$

and:

$$N_{2D}\delta\mathcal{S}_-^{(3)}(\omega_n) = - \int \frac{d^2p}{(2\pi)^2} G_-^{(0)}(\mathbf{p}, \omega_n) G_+^{(0)}(-\mathbf{p}, -\omega_n) G_-^{(0)}(\mathbf{p}, \omega_n) G_+^{(0)}(-\mathbf{p}, -\omega_n),$$

$$N_{2D}\delta\mathcal{S}_+^{(3)}(\omega_n) = \int \frac{d^2p}{(2\pi)^2} G_+^{(0)}(\mathbf{p}, \omega_n) G_-^{(0)}(-\mathbf{p}, -\omega_n) G_+^{(0)}(\mathbf{p}, \omega_n) G_-^{(0)}(-\mathbf{p}, -\omega_n)$$

Note the symmetry property of the (singlet pairing) kernel components:

$$\delta\mathcal{S}_+^{(3)}(\omega_n) = -\delta\mathcal{S}_-^{(3)}(\omega_n), \text{Tr}[\delta\mathcal{S}^{(3)}(\omega_n)] = \delta\mathcal{S}_{\downarrow\uparrow}^{(3)}(\omega_n) - \delta\mathcal{S}_{\uparrow\downarrow}^{(3)}(\omega_n) = 2\delta\mathcal{S}_+^{(3)}(\omega_n)$$

Inserting impurity scattering corrections, bridging pairing vertices, as well as self-energy corrections, we have:

$$N_{2D}\delta\tilde{\mathcal{S}}_{\downarrow\uparrow}^{(3)}(\omega_n) = (|\tilde{\omega}_n| - i\text{sgn}(\omega_n))^3 \int \frac{d^2p}{(2\pi)^2} G_{\downarrow\downarrow}^{(0)}(\mathbf{p}, \tilde{\omega}_n) \tilde{s}_{\downarrow\uparrow}(\omega_n) G_{\uparrow\uparrow}^{(0)}(-\mathbf{p}, -\tilde{\omega}_n)$$

$$\times \tilde{s}_{\uparrow\downarrow}(\omega_n) G_{\downarrow\downarrow}^{(0)}(\mathbf{p}, \tilde{\omega}_n) \tilde{s}_{\downarrow\uparrow}(\omega_n) G_{\uparrow\uparrow}^{(0)}(-\mathbf{p}, -\tilde{\omega}_n),$$

$$N_{2D}\delta\tilde{\mathcal{S}}_{\uparrow\downarrow}^{(3)}(\omega_n) = -(|\tilde{\omega}_n| + i\text{sgn}(\omega_n))^3 \int \frac{d^2p}{(2\pi)^2} G_{\uparrow\uparrow}^{(0)}(\mathbf{p}, \tilde{\omega}_n) \tilde{s}_{\uparrow\downarrow}(\omega_n) G_{\downarrow\downarrow}^{(0)}(-\mathbf{p}, -\tilde{\omega}_n)$$

$$\times \tilde{s}_{\downarrow\uparrow}(\omega_n) G_{\uparrow\uparrow}^{(0)}(\mathbf{p}, \tilde{\omega}_n) \tilde{s}_{\uparrow\downarrow}(\omega_n) G_{\downarrow\downarrow}^{(0)}(-\mathbf{p}, -\tilde{\omega}_n)$$

where:  $G_{\uparrow\uparrow}^{(0)}(\mathbf{p}, \omega_n) \equiv G_-^{(0)}(\mathbf{p}, \omega_n)$ ,  $G_{\downarrow\downarrow}^{(0)}(\mathbf{p}, \omega_n) \equiv G_+^{(0)}(\mathbf{p}, \omega_n)$ , and the two possible vertex renormalization factors,  $\tilde{s}_+(\omega_n) \equiv \tilde{s}_{\downarrow\uparrow}(\omega_n)$ ,  $\tilde{s}_-(\omega_n) \equiv \tilde{s}_{\uparrow\downarrow}(\omega_n)$ , are given by (see Eq.17):

$$\tilde{s}_{\pm}(\omega_n) \approx \frac{|\omega_n| + a_H + b \mp i\text{sgn}(\omega_n)}{(|\omega_n| + a_H)^2 - b^2 + I^2}, a_H \equiv b + 2D(edH/\hbar)^2 \quad (27)$$

Thus, we may rewrite now the linearized cubic term in Eq.24 in the more explicit form:

$$\int d^2r e^{-i\mathbf{q}\cdot\mathbf{r}} \int_0^\beta d\tau e^{i\Omega_\nu\tau} \text{Tr} \left\langle i\sigma_y \delta\mathcal{G}_{21}^{(3)}(\mathbf{r}, \mathbf{r}; \tau, \tau) \right\rangle_{imp}$$

$$\approx 4k_B T (N_{2D}/\hbar^3) \sum_{n=0}^\infty \mathbf{Re} [\tilde{s}_+(\omega_n) |\tilde{s}_+(\omega_n)|^2] \int \frac{d^2q'}{(2\pi)^2} D_T(q') \Delta^*(\mathbf{q}, \Omega_\nu) \quad (28)$$

where  $\tilde{s}_+(\omega_n)$  is given in Eq.27.

We therefore define the finite-field critical shift parameter:

$$\varepsilon_H \equiv \ln(T/T_{c0}) + \frac{1}{2} \left( 1 + \frac{b}{\sqrt{b^2 - I^2}} \right) \psi(1/2 + \overline{\varkappa}_-) + \frac{1}{2} \left( 1 - \frac{b}{\sqrt{b^2 - I^2}} \right) \psi(1/2 + \overline{\varkappa}_+) - \psi(1/2) \quad (29)$$

and expand  $D(q, \Omega_\nu = 0)^{-1}$  (Eq.23) to first order in  $q^2$ , to find:

$$D(q, 0)^{-1} \simeq N_{2D} \left[ \varepsilon_H + \frac{\hbar D}{4\pi k_B T} \eta(H) q^2 \right] \quad (30)$$

where:

$$\eta(H) = \frac{1}{2} \left( 1 + \frac{b}{\sqrt{b^2 - I^2}} \right) \psi' \left( \frac{1}{2} + \bar{\kappa}_- \right) + \frac{1}{2} \left( 1 - \frac{b}{\sqrt{b^2 - I^2}} \right) \psi' \left( \frac{1}{2} + \bar{\kappa}_+ \right) \quad (31)$$

The effect of the interaction term near the critical point can be now included in a modified form of Eq.30, by using Eq.28, i.e.:

$$D_T(q)^{-1} k_B T \simeq N_{2D} \left[ \frac{\varepsilon_H + \frac{\hbar D}{4\pi k_B T} \eta(H) q^2 +}{(4k_B T/\hbar^3) \sum_{n=0}^{\infty} \frac{(\omega_n + a_H + b)[(\omega_n + a_H + b)^2 + I^2]}{[(\omega_n + a_H)^2 - b^2 + I^2]^3}} \int \frac{d^2 q'}{(2\pi)^2} D_T(q') \right] \quad (32)$$

The interaction term includes, as a factor, the thermal fluctuation propagator  $D_T(q')$ , which is proportional to  $1/N_{2D}$ . To take into account the effect of the spin-orbit induced band mixing [7], [8] on the interaction we replace the constant  $N_{2D}$  with a minimal model of piecewise DOS function  $N_{2D}(E)$ , consisting of a relatively heavy electron-band with DOS,  $m^*/2\pi\hbar^2$ , at  $E > E_h$ , and a lighter electron-band at  $E < E_l$ , separated by an energy interval  $E_h - E_l \sim \varepsilon_{SO}$ , in which  $N_{2D}(E) \equiv (m^*/2\pi\hbar^2) \nu(E)$  interpolates between the two pieces (see Fig.(1) in the main text).

### III. SELF-CONSISTENT FIELD APPROXIMATION OF THE INTERACTION BETWEEN FLUCTUATIONS

The thermal fluctuation propagator,  $D_T(q)$ , may be determined by solving numerically the complicated integral equation 32. A much more practical approach is to use the well-known self-consistent field (SCF) approximation, employed e.g. in a similar situation by Ulla and Dorsey in [9]. In this scheme the third term within the large brackets in Eq.32, associated with the linearized cubic term, is absorbed in the field-dependent critical shift parameter  $\varepsilon_H$  to form the interaction-modified critical shift-parameter:

$$\tilde{\varepsilon}_H \equiv \varepsilon_H + (4k_B T/\hbar^3) \sum_{n=0}^{\infty} \mathbf{Re} [\tilde{s}_+(\omega_n)] |\tilde{s}_+(\omega_n)|^2 \int \frac{d^2 q'}{(2\pi)^2} D_T(q') \quad (33)$$

and then, by considering  $D_T(q')$  on the RHS of Eq.32 as a function of  $\tilde{\varepsilon}_H$ :  $D_T(q; \tilde{\varepsilon}_H) \simeq (k_B T/N_{2D}) \left[ \tilde{\varepsilon}_H + \frac{\hbar D}{4\pi k_B T} q^2 \eta(H) \right]^{-1}$ , it can be evaluated by solving Eq.33 for  $\tilde{\varepsilon}_H$ , after replacing there  $D_T(q')$  with  $D_T(q'; \tilde{\varepsilon}_H)$ . The resulting equation, determining  $\tilde{\varepsilon}_H$ , can be conveniently rewritten in terms of the following dimensionless parameters:

$$\delta_0 \equiv \frac{D (deH_{c||0}^*)^2}{2\pi k_B T_c^* \hbar}, \quad \mu_0 \equiv \frac{\mu_B H_{c||0}^*}{2\pi k_B T_c^*}, \quad \beta_0 \equiv \frac{\hbar b}{2\pi k_B T_c^*}, \quad x_0 \equiv \left( \frac{\hbar D q_c^2}{4\pi k_B T_c^*} \right) \quad (34)$$

and the reduced field and temperature,  $h \equiv H/H_{c||0}^*$ ,  $t \equiv T/T_c^*$ , respectively, as:

$$\tilde{\varepsilon}_h = \varepsilon_h + \alpha F(h) \int_0^{x_0 t^{-1}} \frac{dx}{\tilde{\varepsilon}_h/\eta(h) + x} \simeq \varepsilon_h + \alpha F(h) \ln \left( 1 + \frac{\eta(h) x_0}{t \tilde{\varepsilon}_h} \right) \quad (35)$$

where  $T_c^*$  and  $H_{c||0}^*$  are characteristic parameters determining the scales of the transition temperature and the critical parallel field (at zero temperature), respectively,  $x_0 \equiv \hbar D q_c^2 / 4\pi k_B T_c^*$ , where  $q_c$  is a cutoff wavenumber of a fluctuation, and  $\beta \equiv \beta_0/t$ ,  $\mu \equiv \mu_0/t$ ,  $\delta \equiv \delta_0/t$ . The function  $F(h)$  is given by:

$$F(h) = \frac{1}{\eta(h)} \sum_{n=0}^{\infty} \frac{(n+1/2+2\beta+\delta h^2) \left[ (n+1/2+2\beta+\delta h^2)^2 + \mu^2 h^2 \right]}{[(n+1/2+\delta h^2)(n+1/2+2\beta+\delta h^2) + \mu^2 h^2]^3} \quad (36)$$

and  $\alpha$  is given in Eq.3 of the main text.

### IV. FLUCTUATION PARACONDUCTIVITY UNDER A PARALLEL MAGNETIC FIELD

The method of calculation employed here, which was first proposed by Schmidt [10], exploits the TDGL functional  $\mathfrak{L}(\Delta, \mathbf{A})$  of the order parameter  $\Delta(\mathbf{r}, t)$  and the vector potential  $\mathbf{A}(\mathbf{r}, t)$ , to find the Cooper-pairs current density:

$$\mathbf{j}(\mathbf{r}, t) = \frac{\partial \mathfrak{L}(\Delta(\mathbf{r}, t), \mathbf{A}(\mathbf{r}, t))}{\partial \mathbf{A}(\mathbf{r}, t)} \quad (37)$$

A key ingredient in this approach is the inverse fluctuation propagator (in wavevector-frequency representation)  $D^{-1}(\mathbf{q}+2e\mathbf{A}/\hbar, \omega)$ , mediating between the order parameter and the GL functional. In the Gaussian approximation, inherent to the Fulde-Maki approach, the relation is quadratic, i.e.:

$$\mathcal{L}(\Delta, \mathbf{A}) = \left(\frac{1}{2\pi}\right)^2 \int d^2q \left(\frac{1}{2\pi}\right) \int d\omega |\Delta(\mathbf{q}, \omega)|^2 D^{-1}(\mathbf{q}+2e\mathbf{A}/\hbar, \omega)$$

, and the Aslamazov-Larkin time-ordered correlator is given by:

$$Q_{AL}(i\Omega_\nu) = (4eN_{2D}D)^2 d \left(\frac{1}{2\pi}\right)^2 \int d^2q \times k_B T \sum_{\mu=-\infty}^{\infty} q_x^2 C(q, \Omega_\mu + \Omega_\nu) D(q, \Omega_\mu + \Omega_\nu) C(q, \Omega_\mu) D(q, \Omega_\mu) \quad (38)$$

where  $\Omega_\mu = 2\mu k_B T/\hbar$ ,  $\Omega_\nu = 2\nu k_B T/\hbar$ ,  $\mu = 0, \pm 1, \pm 2, \dots$ ,  $\nu = 0, 1, 2, \dots$  are bosonic Matsubara frequencies. Here the electrical current is generated along the  $x$  axis,  $q_z, q_x$  are the fluctuation (in-plane) wave-vector components along the magnetic and electric field directions, respectively,  $q^2 \equiv q_z^2 + q_x^2$ , and  $C(\tilde{q}, \Omega_\mu) \equiv [\partial D^{-1}(\tilde{q}, \Omega_\mu)/\partial A_x]/4DeN_{2D}\tilde{q}_x$ , with  $\tilde{\mathbf{q}} = \mathbf{q} + 2e\mathbf{A}/\hbar$ . Note that in Eq.38 we use for both  $C(q, \Omega_\mu)$  and  $D(q, \Omega_\mu)$  the notations employed in the previous sections for the fluctuation propagator, Eq.23, where the orbital magnetic field effect is implicitly included, whereas in the above definition of  $C(\tilde{q}, \Omega_\mu)$  it is explicit. A simple calculation yields:  $C(q, \Omega_\mu) = \eta(x, y; H)/4\pi k_B T$ , where  $\eta(x, y; H)$  is obtained from  $\eta(H)$ , defined in Eq.31, by replacing  $\mp_\pm$  with  $\mp_\pm + x + y$ . Thus, performing the summation over the bosonic Matsubara frequency  $\Omega_\mu$  in Eq.38 and the analytical continuation  $i\Omega_\nu \rightarrow \omega + i\delta$ , the retarded correlator  $Q_{AL}^R(\omega)$  can be written in the form:

$$Q_{AL}^R(\omega) = k_B T \left(\frac{2e}{\hbar}\right)^2 \left(\frac{1}{2\pi d}\right) \int_0^\infty x dx \sum_{n=0, \pm 1, \pm 2, \dots} \frac{\Phi'(x + |n + y|; \tilde{\varepsilon}_h)}{\Phi(x + |n + y|; \tilde{\varepsilon}_h)} \frac{\Phi'(x + |n|; \tilde{\varepsilon}_h)}{\Phi(x + |n|; \tilde{\varepsilon}_h)} \quad (39)$$

where  $y = \frac{i\hbar\omega}{2\pi k_B T}$ , and:

$$\begin{aligned} \Phi(x + y; \tilde{\varepsilon}_h) &\equiv \tilde{\varepsilon}_h + a_+(h) [\psi(1/2 + f_-(h) + x + y) - \psi(1/2 + f_-(h))] \\ &+ a_-(h) [\psi(1/2 + f_+(h) + x + y) - \psi(1/2 + f_+(h))] \end{aligned}$$

Using Eq.39 the desired static sheet conductivity is readily calculated to be:

$$\sigma_{AL} d = \frac{1}{4} \left(\frac{G_0}{\pi}\right) \int_0^\infty \left(\frac{\Phi'(x; \tilde{\varepsilon}_h)}{\Phi(x; \tilde{\varepsilon}_h)}\right)^2 dx, \quad (40)$$

where  $G_0 = e^2/\pi\hbar$  is the conductance quantum.

## V. DOS CONDUCTIVITY: PHENOMENOLOGICAL VS. MICROSCOPIC APPROACH

In this section we will show that the result for the DOS conductivity derived in the main text using a phenomenological approach based on the simple Drude formula is, to a good approximation, equal to the result derived by Larkin-Varlamov [11] by means of a microscopic (diagrammatic) approach in the dirty limit.

For the sake of simplicity of the comparison we consider the electron gas model without spin. In the phenomenological approach we use in the Drude formula:  $\delta\sigma^{DOS} = -2n_s e^2 \tau_{SO}/m^*$ , the fluctuation Cooper-pair density  $n_s = d^{-1} (2\pi)^{-2} \int d^2q \langle |\psi(q)|^2 \rangle$ , with the momentum distribution in the dirty limit:

$$\langle |\psi(q)|^2 \rangle = \left(\frac{2E_F}{\pi^2 k_B T}\right) \frac{1}{\ln \frac{T}{T_{co}} + \frac{\hbar D}{4\pi k_B T} q^2} \quad (41)$$

Performing the integration:  $n_s = \frac{1}{d} \frac{1}{\hbar D} \left(\frac{2E_F}{\pi^2}\right) \int_0^{x_c} dx \frac{1}{\varepsilon + x}$ , where  $x_c \equiv x_0/t$ , the DOS conductivity is:

$$\delta\sigma^{DOS} d \simeq -0.4 \left(\frac{e^2}{\hbar}\right) \ln\left(\frac{x_c}{\varepsilon}\right) \quad (42)$$

The corresponding result of the microscopic calculation, which includes all diagrams contributing to the DOS conductivity [11]:

$$\delta\sigma_{xx}^{DOS} \simeq -\frac{e^2}{2d\hbar} \kappa(k_B T \tau / \hbar) \ln\left(\frac{x_c}{\varepsilon}\right)$$

In the dirty limit,  $k_B T \ll \hbar/\tau$ ,  $\kappa(k_B T \tau / \hbar) \rightarrow 56\zeta(3)/\pi^4 \simeq 0.7$ , and:

$$\delta\sigma_{xx}^{DOS} d \simeq -0.35 \left(\frac{e^2}{\hbar}\right) \ln\left(\frac{x_c}{\varepsilon}\right) \quad (43)$$

in good agreement with 42.

## VI. LIMITING RESULTS OF THE TOTAL SHEET CONDUCTANCE

The *thermal limit* of the total sheet conductance (compare Eq.8 of the main text in the limit  $T_Q \rightarrow 0$ ) takes the form:

$$\begin{aligned} \sigma d &= (\sigma_n + \delta\sigma_{DOS} + \sigma_{AL}) d \\ &= \sigma_n d + \left(\frac{G_0}{\pi}\right) \left[ \frac{1}{4} \int_0^{x_c} \left( \frac{\Phi'(x; \tilde{\varepsilon}_h)}{\Phi(x; \tilde{\varepsilon}_h)} \right)^2 dx - 4 \int_0^{x_c} \Phi^{-1}(x; \tilde{\varepsilon}_h) dx \right] \end{aligned} \quad (44)$$

In the absence of the self-consistent interaction term in Eq.35, both the Aslamozov-Larkin  $\sigma_{AL}$  and the DOS conductivity  $\delta\sigma_{DOS}$  diverge at some critical field,  $H_{c\parallel}$ , reflecting the divergence of the free (Gaussian) fluctuation propagator  $1/\Phi(x; \varepsilon_h) N_{2D}$  at  $\varepsilon_h = 0$ ,  $x = 0$ . However, since the divergence of the positively defined  $\sigma_{AL}$  is much stronger than that of the negatively defined  $\delta\sigma_{DOS}$ , it turns on a macroscopic superconducting order established below  $H_{c\parallel}$ . On the other hand, since  $\delta\sigma_{DOS}$  is typically much larger in magnitude than  $\sigma_{AL}$ , except near  $H_{c\parallel}$  (where the divergence of  $\sigma_{AL}$  is stronger than that of  $\delta\sigma_{DOS}$ ), the total sheet resistance  $\rho/d \equiv 1/\sigma d$  is larger than its asymptotic limit  $1/\sigma_n d$  in a broad fields range above  $H_{c\parallel}$ , consequently showing a MSR peak above the superconducting transition.

Results of calculations of the sheet resistance as a function of the magnetic field, for different temperatures, based on Eq.44 in the presence of the self-consistent interaction term, are shown in Fig.(1), together with experimental data presented in [12]. In the calculation the smearing of the sharp transition to zero resistivity, predicted by the simple Gaussian-fluctuations approximation, is due to the effect of the interaction term in Eq.35. As shown in Fig.(2) of the main text, all solutions of the SCF equation 35 satisfy  $\tilde{\varepsilon}_h > 0$ , implying that the critical divergence of the free fluctuations propagator is strictly removed. Thus, for the temperatures above and near  $T_c$  ( $\approx 212$  mK) the calculated MSR agree quite well with the experimental data. However, upon reducing the temperature below  $T_c$  the agreement quickly deteriorates so that for the lowest temperature ( $T = 30$  mK) shown in Fig.(1), the MSR peak is much too sharp as compared to the experimental data.

The *quantum limit* of the sheet conductivity, i.e. the  $T \rightarrow 0$  limit of Eq.8 of the main text, should be carefully checked to ensure it is physically meaningful at very low temperatures. Let us start with the quantum limit ( $T \rightarrow 0, \varsigma \equiv T_Q/2T \rightarrow \infty$ ) of the unified versions of the functions  $\varepsilon_h$  and  $\eta(h)$ , i.e.:

$$\varepsilon_h^U \equiv \ln(T/T_{c0}) + \left[ \frac{a_+(h) \psi(1/2 + \varsigma + f_-(h)) + a_-(h) \psi(1/2 + \varsigma + f_+(h))}{a_-(h) \psi(1/2 + \varsigma + f_+(h))} \right] - \psi(1/2), \quad (45)$$

$$\eta_U(h) \approx \sum_{n=0}^{\infty} \frac{(n + 1/2 + \varsigma + 2\beta + \delta h^2)^2 - \mu^2 h^2}{[(n + 1/2 + \varsigma + \delta h^2)(n + 1/2 + \varsigma + 2\beta + \delta h^2) + \mu^2 h^2]^2} \quad (46)$$

The  $T \rightarrow 0$  limit of  $\varepsilon_h^U$  is calculated by exploiting the identity  $\sum_{n=0}^{n_c} 1/(n + 1/2) = -\psi(1/2) + \psi(n_c + 3/2)$  in conjunction with the asymptotic expansion of the digamma function  $\psi(z)$  to find:

$$\begin{aligned} \varepsilon_h^Q &\equiv (\varepsilon_h^U)_{\varsigma \rightarrow \infty} \approx \ln\left(\frac{2e^\gamma T_Q}{T_{c0}}\right) + \delta^{(1)} \varepsilon_h^Q, \\ \delta^{(1)} \varepsilon_h^Q &= \frac{1}{2} \left\{ \ln\left[\frac{(1/2 + \delta_Q h^2)(1/2 + 2\beta_Q + \delta_Q h^2) + \mu_Q^2 h^2}{\sqrt{\beta_Q^2 - \mu_Q^2 h^2}}\right] + \frac{\beta_Q}{\sqrt{\beta_Q^2 - \mu_Q^2 h^2}} \ln\left(\frac{1/2 + \beta_Q + \delta_Q h^2 - \sqrt{\beta_Q^2 - \mu_Q^2 h^2}}{1/2 + \beta_Q + \delta_Q h^2 + \sqrt{\beta_Q^2 - \mu_Q^2 h^2}}\right) \right\} + \ln 2 \end{aligned} \quad (47)$$



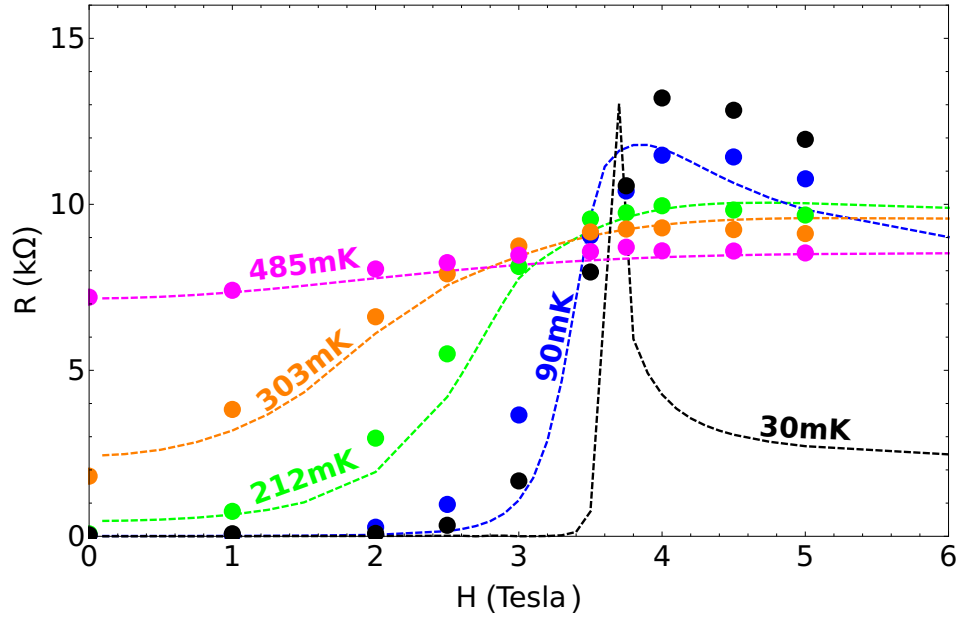

FIG. 1 Calculated sheet resistance as a function of field  $H$ , obtained by using Eq.44, for  $R_N = 7.5\text{k}\Omega$ , and for different temperatures (dashed lines), plotted together with the corresponding experimental data (full circles) extracted from Ref. [12]. The fitting parameters are (see Eq.34):  $T_{c0} = .4\text{K}$ ,  $\beta_0 = 8$ ,  $\alpha = .1$ ,  $\delta_0 = .028$ ,  $x_0 = .1$ . Note the quick narrowing of the MSR peak for decreasing temperature below  $T_c$  ( $\sim 212\text{ mK}$ ).

where  $\gamma = 0.57721\dots$ , and:

$$\tilde{\delta}_Q \equiv \frac{D \left( deH_{c||0}^* \right)^2}{2\pi k_B T_Q \hbar}, \quad \mu_Q \equiv \frac{\mu_B H_{c||0}^*}{2\pi k_B T_Q}, \quad \beta_Q \equiv \frac{\hbar b}{2\pi k_B T_Q}$$

For  $\eta_U(h)$ , we use the expression 46 to show that:

$$(\eta_U(h))_{t \rightarrow 0} = \left( \frac{1}{2\varsigma} \right)_{\varsigma \rightarrow \infty} \eta_Q(h) \quad (48)$$

where:

$$\eta_Q(h) \equiv \int_0^\infty d\nu \frac{(\nu + 1/2 + 2\beta_Q + \delta_Q h^2)^2 - \mu_Q^2 h^2}{\left[ (\nu + 1/2 + \delta_Q h^2)(\nu + 1/2 + 2\beta_Q + \delta_Q h^2) + \mu_Q^2 h^2 \right]^2} \quad (49)$$

In evaluating the quantum limit of the interaction term;

$$\delta^{(3)} \varepsilon_h^U \equiv \alpha F_U(h) (1 + 2\varsigma) \ln \left( 1 + \frac{x_0 \eta_U(h) t^{-1}}{\tilde{\varepsilon}_h^U} \right) \quad (50)$$

(see Eq.35 and Eq.4 of the main text) we focus first on the distribution function:

$$F_U(h) = \frac{1}{\eta_U(h)} \sum_{n=0}^\infty \frac{(n + 1/2 + \varsigma + 2\beta + \delta h^2) \left[ (n + 1/2 + \varsigma + 2\beta + \delta h^2)^2 + \mu^2 h^2 \right]}{\left[ (n + 1/2 + \varsigma + \delta h^2)(n + 1/2 + \sigma + 2\beta + \delta h^2) + \mu^2 h^2 \right]^3} \quad (51)$$

We find the limiting relation:

$$(F_U(h))_{t \rightarrow 0} = \left( \frac{1}{2\varsigma} \right)_{\varsigma \rightarrow \infty} F_Q(h)$$

where:

$$F_Q(h) \equiv \frac{1}{\eta_Q(h)} \int_0^\infty d\nu \frac{(\nu + 1/2 + \varsigma + 2\beta_Q + \delta_Q h^2) \left[ (\nu + 1/2 + \varsigma + 2\beta_Q + \delta_Q h^2)^2 + \mu_Q^2 h^2 \right]}{\left[ (\nu + 1/2 + \varsigma + \delta_Q h^2) (\nu + 1/2 + \varsigma + 2\beta_Q + \delta_Q h^2) + \mu_Q^2 h^2 \right]^3}$$

implying that in the quantum limit  $(F_U(h))_{t \rightarrow 0}$  vanishes like  $(1/2\varsigma)_{\varsigma \rightarrow \infty}$ . However, due to the divergent factor  $(1 + 2\varsigma)$ , the product  $F_U(h) (1 + 2\varsigma)$  remains finite. Furthermore, the function  $\eta_U(h)$ , which appears in the argument of the logarithm in Eq.50 (as well as the logarithm itself), vanishes in the quantum limit, see Eq.48.

Nevertheless, the limiting logarithm does not vanish, since:  $x_0 \eta_U(h) t^{-1} \rightarrow x_0 \eta_Q(h) (T/T_Q)_{T \rightarrow 0} t^{-1} = x_0 \eta_Q(h) t_Q^{-1}$ , where  $t_Q \equiv T_Q/T_{c0}^*$ . Combining all the limiting terms in Eq.50, the total interaction correction also remains finite in the quantum limit, i.e.:

$$\left( \delta^{(3)} \varepsilon_H^U \right)_{T \rightarrow 0} = \alpha F_Q(h) \ln \left( 1 + \frac{x_0 t_Q^{-1} \eta_Q(h)}{\varepsilon_h^Q} \right) \quad (52)$$

The strict cancellation of the divergent fluctuation-propagator with the vanishing electronic correlation-function in the zero temperature limit, outlined above, reflects the consistency of the two elements introduced to our unified QT fluctuations approach: The excess quantum-tunneling "temperature",  $T_Q$ , in the fluctuation propagator, as defined in the main text, and the bosonic Matsubara frequency-shift in the electronic pair-correlation function  $s_+(\omega_n)$ .

Finally, let us check the quantum limit of the unified QT sheet conductivity,  $\sigma^U d$  (see Eq.8 in the main text). To do so we exploit the small momentum expansion of the fluctuation propagator, namely the linear approximation  $\Phi(x; \tilde{\varepsilon}_h) \simeq \tilde{\varepsilon}_h + \eta(h)x$  in the calculations of both the AL and DOS conductivities, which enables analytical evaluation of the integrations. Thus, starting with the AL contribution we evaluate:  $(1/4) \int_0^{t^{-1}x_0} [\Phi'(x; \tilde{\varepsilon}_h) / \Phi(x; \tilde{\varepsilon}_h)]^2 dx \simeq$

$\eta(h) / [4\tilde{\varepsilon}_h (1 + t\tilde{\varepsilon}_h/x_0\eta(h))]$ , whereas for the DOS contribution we find:  $-4 \int_0^{t^{-1}x_0} \Phi(x)^{-1} dx \simeq -(4/\eta(h)) \ln [1 + x_0\eta(h)/t\tilde{\varepsilon}_h]$ . Using the above integrals, we get for the sheet conductance in the unified QT fluctuation framework:

$$\sigma^U d \approx \sigma_n d + \left( \frac{G_0}{\pi} \right) \left[ \frac{1}{4} \frac{\left( 1 + \frac{T_Q}{T} \right) \eta_U(h)}{\tilde{\varepsilon}_h^U \left( 1 + \frac{t\tilde{\varepsilon}_h^U}{x_0\eta_U(h)} \right)} - 4 \frac{\ln \left( 1 + \frac{x_0\eta_U(h)}{t\tilde{\varepsilon}_h^U} \right)}{\left( 1 + \frac{T_Q}{T} \right) \eta_U(h)} \right] \quad (53)$$

Now, in the quantum limit:  $[\eta_U(h)]_{T \rightarrow 0} = (T/T_Q)_{T \rightarrow 0} \eta_Q(h)$ , so that:  $[(1 + T_Q/T) \eta_U(h)]_{T \rightarrow 0} = \eta_Q(h)$ , and also:  $[x_0\eta_U(h)/t\tilde{\varepsilon}_h^U]_{T \rightarrow 0} = x_0\eta_Q(h)/t_Q\tilde{\varepsilon}_h^Q$ , yielding the final, finite non-singular result:

$$\sigma^Q d \approx \sigma_n d + \left( \frac{G_0}{\pi} \right) \left[ \frac{1}{4} \frac{\eta_Q(h)}{\tilde{\varepsilon}_h^Q \left( 1 + \frac{t_Q\tilde{\varepsilon}_h^Q}{x_0\eta_Q(h)} \right)} - 4 \frac{\ln \left( 1 + \frac{x_0\eta_Q(h)}{t_Q\tilde{\varepsilon}_h^Q} \right)}{\eta_Q(h)} \right] \quad (54)$$

## VII. THE FITTING PROCESS

As explained in [12], since labeling each data set according to the measured gate voltage  $V_g$  is not a unique procedure, they are instead labeled by  $R_N$ -the corresponding sheet resistance measured at zero field and sufficiently high temperature ( $T = 1\text{K}$ ). Thus, focusing on three representative  $R_N$  values (see Table I) of the extensive experimental sheet-resistance data reported in Ref.[12], we have exploited the data provided in Ref.[13] to select values for the basic (gate-voltage dependent) microscopic parameters of our theoretical model;  $\beta_0(R_N) \equiv \varepsilon_{SO}(R_N)/4\pi k_B T_c^*$ , and  $\delta_0(R_N) \equiv D(R_N) \left( deH_{c||0}^* \right)^2 / 2\pi k_B T_c^* \hbar$ , where  $H_{c||0}^* = 4.5\text{T}$  is a characteristic scale for the critical field at zero temperature, and  $T_c^* = 0.212\text{K}$  is a characteristic scale for the transition temperature. The dimensionless Zeeman splitting parameter  $\tilde{I}_0 \equiv \mu_B H_{c||0}^* / 2\pi k_B T_c^*$ , was selected to coincide with the free-electron value:  $\tilde{I}_0 = 2.4$ . Given the uncertainty involved in determining the numerical values of  $\varepsilon_{SO}(R_N)$  from the current literature, we allow for some freedom in their selection in order to facilitate the fitting process.

The key interaction parameter  $\alpha(R_N)$  (see Eq.(3) in the main text) is related to  $\beta_0(R_N)$  through:

$$\alpha(R_N) = \frac{\alpha_0}{\kappa(R_N)\nu(E_F)} \quad (55)$$

where:

$$\kappa(R_N) \equiv \frac{\eta_{2D}(R_N)}{\beta_0(R_N)} \quad (56)$$

$\alpha_0 = 2/\pi^3 = 0.0645$ ,  $\eta_{2D}(R_N) \equiv \hbar^2 n_{2D}(R_N) / 4\pi m^* k_B T_c^*$ , and  $n_{2D}(R_N) = k_F^2 / 2\pi$  is the effective interface carrier density, with  $k_F$ -the Fermi wavenumber.

Another important, gate-voltage dependent parameter is the dimensionless cutoff  $x_0 \equiv (T/T_c^*) x_c$ . Its evaluation (through  $q_c$ ) is beyond the scope of our theory, however its dependence on the gate voltage can be expressed through the connecting function  $\kappa(R_N)$  (Eq.56), i.e.:

$$x_0(R_N) = \tilde{x}_0 \kappa(R_N) \quad (57)$$

where  $\tilde{x}_0 \equiv E_c / 2k_B T_c^*$  is a free adjustable parameter (best fitting value:  $\tilde{x}_0 = 0.015$ ), independent of  $R_N$ , with  $E_c \equiv \hbar^2 q_c^2 / 2m^*$ . Its value influences mainly the high field behavior through the DOS conductivity, and its optimal selection is closely connected to the selected value of the normal state conductivity parameter  $\sigma_n$ .

A similar dependence on  $R_N$  characterizes the dimensionless diamagnetic energy parameter  $\delta_0 \equiv (T/T_c^*) \delta$ , i.e.:

$$\delta_0(R_N) = \tilde{\delta}_0 \kappa(R_N) \quad (58)$$

where  $\tilde{\delta}_0 \equiv E_d / 2k_B T_c^*$  and  $E_d \equiv (deH_{c||0}^*)^2 / m^*$  is the diamagnetic energy  $E_d$ , which depends on the effective width of the interface region. The latter contains only a few atomic layers so that  $d \sim 1nm$ .

The mean-field transition temperature at zero field,  $T_{c0}$  is treated here as an adjustable parameter (best fitting value:  $T_{c0} = 0.43K$ ) due to the lack of detailed microscopic calculations of the basic SC parameters characterizing the complex  $LaAlO_3/SrTiO_3$  (111) interface.

The best fitting values of the spin-orbit energy parameter  $\varepsilon_{SO}(R_N)$  (see Table I), obtained in our fitting process, decrease monotonically with the decreasing values of the gate voltage  $V_g$  (or the increasing values of  $R_N$ ) on the LHS of the dome-shaped curve of  $\varepsilon_{SO}$  vs.  $V_g$  shown in Ref.[13]. The magnitude of the largest fitted value of  $\varepsilon_{SO}$  (i.e.  $3.2meV$  at  $R_N = 7.5k\Omega$ ) is by a factor of 2 smaller than the maximum found in [13] on the basis of mean-field calculation of the critical field  $H_{c||}$  vs.  $\varepsilon_{SO}$  and its determination vs.  $V_g$  from resistivity measurements. The differences are likely to be due to the failure of the mean-field approximation in the fluctuation-controlled phenomenon under study.

Thus, examining the sheet-resistance data presented in [12], we may roughly identify  $\varepsilon_{SO}(7.5k\Omega)$  with the top of the dome-shaped  $\varepsilon_{SO}$  vs.  $V_g$  curve shown in [13]. This enables us to start constructing the DOS function  $N_{2D}(E)$  from the best fitting parameters  $\alpha(R_N)$  (Eq.55) and  $\kappa(R_N)$  (Eq.56). Exploiting Eq.(3) of the main text, one may find  $N_{2D}(E_F)$  from the values of  $\alpha(R_N)$ , provided the diffusion coefficient  $D$  is known. The latter:  $D \approx 1.8 \times 10^{-4} m^2/s$ , is found by exploiting the weak antilocalisation relation:  $eD = \varepsilon_{SO}(R_N) / 4H_{SO}(R_N)$  [13] (with  $H_{SO}$ - the spin-orbit field, estimated to be about 4.5T at  $R_N = 7.5k\Omega$ ), and our best fitting value for  $\varepsilon_{SO}(7.5k\Omega) \simeq 3.2meV$ . Assuming for the range of the  $R_N$  values investigated, that  $\varepsilon_{SO}(R_N)$  is a linear function of the carrier density  $n_{2D}(R_N)$ , we have found the best fitting value  $\kappa(R_N) \equiv \kappa = 0.8$ . These results enable us finding numerical estimates for both the carrier density  $n_{2D}$  and the effective mass  $m^*$  by solving the consequent coupled equations:

| $R_N[k\Omega]$ | $\beta_0$ | $\alpha$ | $\nu(E_F)$ | $\varepsilon_{SO}[meV]$ | $n_{2D}[cm^{-2}]$    | $E_F[meV]$ |
|----------------|-----------|----------|------------|-------------------------|----------------------|------------|
| 7.5            | 14        | .09      | 1.00       | 3.2                     | $.55 \times 10^{13}$ | 8.2        |
| 10.5           | 12.5      | .11      | .77        | 2.87                    | $.48 \times 10^{13}$ | 7.2        |
| 20.5           | 11        | .30      | .29        | 2.52                    | $.43 \times 10^{13}$ | 6.5        |

TABLE I Values of the basic microscopic parameters of the model extracted in the fitting process from the experimental sheet resistance data reported in Ref.[12] for three values of  $R_N$ .

| $R_N = 7.5[k\Omega]$ |           |          |          | $R_N = 10.5[k\Omega]$ |           |          |          | $R_N = 20.5[k\Omega]$ |           |          |          |
|----------------------|-----------|----------|----------|-----------------------|-----------|----------|----------|-----------------------|-----------|----------|----------|
| $T[mK]$              | $T_q[mK]$ | $H_q[T]$ | $H_n[T]$ | $T[mK]$               | $T_q[mK]$ | $H_q[T]$ | $H_n[T]$ | $T[mK]$               | $T_q[mK]$ | $H_q[T]$ | $H_n[T]$ |
| 30                   | 78        | 8        | 6        | 30                    | 80        | 7.3      | 5.5      | 30                    | 89        | 6.5      | 3        |
| 90                   | 70        | 10       | 8        | 130                   | 68        | 10       | 6        | 121                   | 81        | 7        | 3.5      |
| 212                  | 52        | 20       | 12       | 230                   | 56        | 15       | 8        | 212                   | 72        | 8        | 5        |
| 303                  | 40        | 25       | 14       | 330                   | 45        | 18       | 9        | 303                   | 60        | 10       | 6.5      |
| 485                  | 0         | 30       | 20       | 430                   | 22        | 25       | 12       | 394                   | 50        | 20       | 8        |

TABLE II Values of the parameters extracted in the fitting process, which determine the temperature and field dependencies of the normal-state MR and of the quantum tunneling attempt rate  $T_Q$ , for the different values of  $R_N$ .

$$\frac{\hbar^2 n_{2D}}{m^* \varepsilon_{SO}} = \kappa = 0.8, \quad (59)$$

$$\pi \frac{\hbar^3 n_{2D}}{\varepsilon_{SO} m^{*2}} = D = 1.8 \times 10^{-4} \left( \frac{m^2}{s} \right) \quad (60)$$

yielding:  $n_{2D}(7.5k\Omega) \simeq 0.55 \times 10^{13} cm^{-2}$ , and:  $m^* \simeq 1.6m_e$ , where  $m_e$  is the free-electron mass.

An independent determination of the effective mass  $m^*$ , which provides a self-consistent test of the fitting procedure, can be made by exploiting Eq.(3) of the main text with the best fitting values of  $\nu(E_F)$  and  $\alpha(R_N)$  at  $R_N = 7.5k\Omega$ , together with the weak antilocalisation value of  $D$  found above. The resulting equation for  $m^*$ , after substituting the best fitting values:  $\nu(E_F) = 1$  and  $\kappa = 0.8$  in Eq.55, reads:  $2\hbar/\pi^2 D m^* = 0.0875$ , where  $D \approx 1.8 \times 10^{-4} m^2/s$ . The result;  $m^* \simeq 1.5m_e$ , agrees quite well with the value found above.

Furthermore, it is also found to be in very good agreement with the cyclotron effective mass ( $m_c^* = 1.6m_e$ ) reported in Ref.[8] using Shubnikov-de Haas (SdH) oscillations measurement.

Our next step in constructing the DOS function  $N_{2D}(E)$  is to exploit the best fitting values of  $\alpha(R_N)$  for the different values of  $R_N$  investigated (with  $\kappa = 0.8$ ) in Eq.55, and then extract the corresponding values of  $\nu(E_F)$  (see Table I). The corresponding values of the carrier density and Fermi energy can be found from the respective relations:

$$n_{2D}(R_N) = 4\pi \frac{m^* k_B T_c^*}{\hbar^2} \kappa \beta_0(R_N), \quad (61)$$

$$E_F(R_N) = \pi \frac{\hbar^2 n_{2D}(R_N)}{m^*} \quad (62)$$

Comparing the results for the carrier density  $n_{2D}(R_N)$ , shown in Table I, to the data reported in Ref.[12] for the measured inverse Hall coefficient  $e/R_H \equiv n_{2D}^{Hall}(R_N)$  we find the former smaller than the latter by one to two orders of magnitude. However, the values of  $n_{2D}(R_N)$  shown in Table I (i.e.  $\sim 0.5 \times 10^{13} cm^{-2}$ ) are seen to be in good agreement with the sheet carrier density  $n_{2D}^{SdH}$ , determined from the SdH oscillations measurements, reported in Ref.[8]. The large difference between the carrier densities extracted from the two methods could attributed to contributions to transport of at least two bands with different mobilities (see the main text for the detailed explanation).

The dimensionless diamagnetic energy,  $\delta_0(R_N)$ , can be used for determining the effective film thickness  $d$  in our model, in order to estimate the width of the actual interface. So using the diffusion coefficient  $D \approx 1.8 \times 10^{-4} m^2/s$  and our fitting value,  $\delta_0(7.5k\Omega) = 0.028$  ( $\tilde{\delta}_0 = 0.035$ ), in the above expression for  $\delta_0(R_N)$ , we find for the film thickness  $d \approx 0.8nm$ , which is quite a reasonable result.

The normal-state conductivity contribution  $\sigma_n(H, T)$ , defined in the main text with the two adjustable parameters  $\sigma_0$ , and  $H_n(T)$  (see table II), can be tested vs. the negative MR observed in Ref.[14], and [7]. Using the usual definition of the MR, i.e.:  $MR(H, T) \equiv [\rho_n(H, T) - \rho_n(0, T)]/\rho_n(0, T)$ , where  $\rho_n(H, T) = 1/\sigma_n(H, T)$ , our model yields the expression:

$$MR(H, T) = - \frac{(H/H_n(T))^2}{1 + (H/H_n(T))^2} \quad (63)$$

which is plotted in Fig.(3) of the main text for the different  $R_N$  values investigated here.

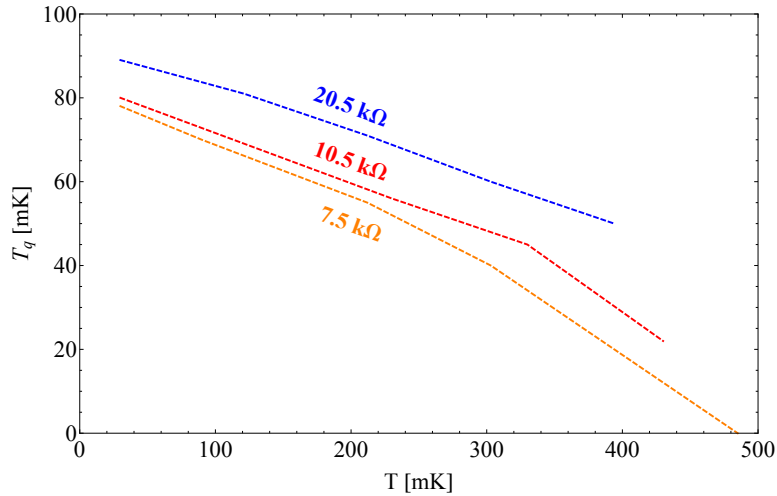

FIG. 2 Tunneling attempt rate  $T_Q$  vs.  $T$  for  $R_N = 7.5, 10.5$ , and  $20.5 k\Omega$ , plotted on the basis of Eq.64 by using the parameters shown in Table II.

Finally, the large body of experimental data analyzed in our fitting process enables us to determine the temperature and field dependence of the phenomenological quantum tunneling "temperature" parameter  $T_Q(T, H)$ . For the field dependence we have selected a particular form, i.e.:

$$T_Q(T, H) = T_Q(T) \left[ 1 - \left( \frac{H}{H_Q(T)} \right)^2 \right] \quad (64)$$

which reflects the expected [15] decreasing quadratic dependence of the superconducting order parameter on increasing field (See table II for the values of  $T_Q(T)$  and  $H_Q(T)$ ). The temperature dependence at zero field,  $T_Q(T)$ , for the three values of  $R_N$ , is shown in Fig.( 2 ). It is seen to qualitatively follow the expected decreasing order parameter with increasing temperature, that would have been measured locally within a superconducting fluctuation-puddle. The somewhat larger values of  $T_Q(T)$  at larger  $R_N$ , which reflect larger tunneling attempt frequency of fluctuations across GL energy barriers, seems to be a reasonable outcome of the respective larger interaction coupling constant  $\alpha$  between Gaussian fluctuations.

### VIII. LOCALIZATION AND THE SHEET RESISTANCE-PEAK AT HIGH FIELDS

To investigate Cooper-pairs localization in the sheet-resistance peak region we consider the Cooper-pairs amplitude correlation function:  $\langle \psi^*(\mathbf{r}) \psi(\mathbf{r} + \rho) \rangle$  (that is proportional to the static fluctuation propagator in real space, see Eq.30):

$$g(\rho) \equiv \langle \psi^*(\mathbf{r}) \psi(\mathbf{r} + \rho) \rangle = \left( \frac{1}{2\pi} \right)^2 \int d^2q \langle |\psi(q)|^2 \rangle e^{i\mathbf{q} \cdot \rho}$$

Performing the angular integration:  $\langle \psi^*(\mathbf{r}) \psi(\mathbf{r} + \rho) \rangle = (2\pi)^{-1} \int_0^{q_c} q dq \langle |\psi(q)|^2 \rangle J_0(q\rho)$ , and using the explicit expression (see Eq.41):  $\langle |\psi(q)|^2 \rangle \simeq (2E_F/\pi^2 k_B T) \Phi^{-1}(x; \tilde{\varepsilon}_h) \approx (2E_F/\pi^2 k_B T) [\tilde{\varepsilon}_h + \eta(h)x]^{-1}$ , with  $x = \hbar D q^2 / 4\pi k_B T$ , we have:

$$\langle \psi^*(\mathbf{r}) \psi(\mathbf{r} + \rho) \rangle \approx \left( \frac{4E_F}{\hbar D \eta(h) \pi^2} \right) \int_0^{q_c} \frac{q dq}{\xi_h^{-2} + q^2} J_0(q\rho)$$

where:

$$\xi_h = \sqrt{\frac{\hbar D}{4\pi k_B T} \frac{\eta(h)}{\tilde{\varepsilon}_h}} \quad (65)$$

is the fluctuations correlation length. The prefactor is rewritten in the form:  $4E_F/\hbar D \eta(h) \pi^2 = 4\varepsilon_{SO} n_{2D}/\pi \eta(h) E_F$ , so that:

$$g(\rho) \simeq \frac{4}{\pi \eta(h)} \left( \frac{\varepsilon_{SO}}{E_F} \right) n_{2D} \int_0^{q_c} \frac{q dq}{\xi_h^{-2} + q^2} J_0(q\rho) \quad (66)$$

Note that the superfluid density is:

$$n_s = \langle |\psi(\mathbf{r})|^2 \rangle = g(0) \simeq (2\varepsilon_{SO} n_{2D}/\pi \eta(h) E_F) \int_0^{q_c} (\xi_h^{-2} + q^2)^{-1} d(q^2):$$

$$n_s = g(0) \simeq \frac{2}{\pi \eta(h)} \left( \frac{\varepsilon_{SO}}{E_F} \right) n_{2D} \ln [1 + (q_c \xi_h)^2] \quad (67)$$

The spatial uniformity of the superfluid density  $g(0) = \langle |\psi(\mathbf{r})|^2 \rangle$  is due to the averaging over the fluctuations configurations. The underlying structure of superconducting puddles is revealed by the correlation function  $g(\rho) = \langle \psi^*(\mathbf{r}) \psi(\mathbf{r} + \rho) \rangle$ , Eq.66. It is proportional to the probability amplitude for Cooper-pair fluctuation at any point  $\mathbf{r}$  to propagate a distance  $\rho$  from  $\mathbf{r}$ . Its dependence on  $\rho$  has a decaying envelope modulated by an oscillatory function associated with the sharp cutoff  $q_c$ . The length scale of this attenuation is the correlation length  $\xi_h$  (Eq.65), which can also be regarded as a length of localization of Cooper-pair fluctuations.

The dependence of  $\xi_h$  on the field  $H$  is through the interaction-modified critical shift parameter  $\tilde{\varepsilon}_h$  and the correction to the stiffness parameter  $\eta(h)$ . Note that by increasing the field  $H$  toward the sheet-resistance peak region the gap  $\tilde{\varepsilon}_h$  in the fluctuation spectrum significantly increases whereas the stiffness  $\eta(h) \hbar D/4\pi k_B T$  decreases (see Figs.(3a,b)), both resulting in a smaller localization length  $\xi_h$  (see Fig.(3c)). The field dependence of the superfluid density, Eq.67, in the sheet-resistance peak region is dominated by the decreasing argument of the logarithm (i.e.  $1 + (q_c \xi_h)^2$ ) upon decreasing  $\xi_h$ . In this region  $(q_c \xi_h)^2 \ll 1$ , so that:

$$n_s \approx \frac{2}{\pi} \left( \frac{\varepsilon_{SO}}{E_F} \right) n_{2D} \frac{\hbar D q_c^2}{4\pi k_B T} \frac{1}{\tilde{\varepsilon}_h}$$

showing that the field dependence of  $n_s$  in this region is mainly controlled by  $\tilde{\varepsilon}_h$ .

In the presence of quantum tunneling, i.e. for a finite  $T_Q$ , one finds:

$$\begin{aligned} \langle \psi^*(\mathbf{r}) \psi(\mathbf{r} + \rho) \rangle &\rightarrow (2\pi)^{-1} [2E_F/\pi^2 k_B (T + T_Q)] \int_0^{q_c} [\tilde{\varepsilon}_h^U + \hbar D \eta_U(h) q^2/4\pi k_B T]^{-1} q dq J_0(q\rho) \\ &= [4E_F/\hbar D (1 + T_Q/T) \eta_U(h) \pi^2] \int_0^{q_c} [(\xi_h^U)^{-2} + q^2]^{-1} q dq J_0(q\rho), \text{ with:} \end{aligned}$$

$$\xi_h^U = \rho_0 \sqrt{\frac{\eta_U(h)}{\tilde{\varepsilon}_h^U}} \quad (68)$$

where  $\rho_0 \equiv \sqrt{\hbar D/4\pi k_B T}$ , and:

$$g_U(\rho) \simeq \frac{4}{\pi (1 + T_Q/T) \eta_U(h)} \left( \frac{\varepsilon_{SO}}{E_F} \right) n_{2D} \int_0^{q_c} \frac{q dq}{(\xi_h^U)^{-2} + q^2} J_0(q\rho) \quad (69)$$

Thus, quantum tunneling of Cooper-pairs increases  $\tilde{\varepsilon}_h$  and diminishes  $\eta(h)$ , implying shortening of the localization length by tunneling (see Fig.(3c)). This also implies suppressed superfluid density due to tunneling (Fig. 3c), which is consistent with the tendency of phase slips to suppress superconducting order.

In the quantum limit, where  $[\eta_U(h)]_{T \rightarrow 0} = (T/T_Q) \eta_Q(h) \rightarrow 0$ , we find:

$$\xi_h^Q \equiv \left( \frac{\hbar D}{4\pi k_B T} \frac{\eta_U(h)}{\tilde{\varepsilon}_h^U} \right)_{T \rightarrow 0}^{1/2} = \sqrt{\frac{\hbar D}{4\pi k_B T_Q} \frac{\eta_Q(h)}{\tilde{\varepsilon}_h^Q}}$$

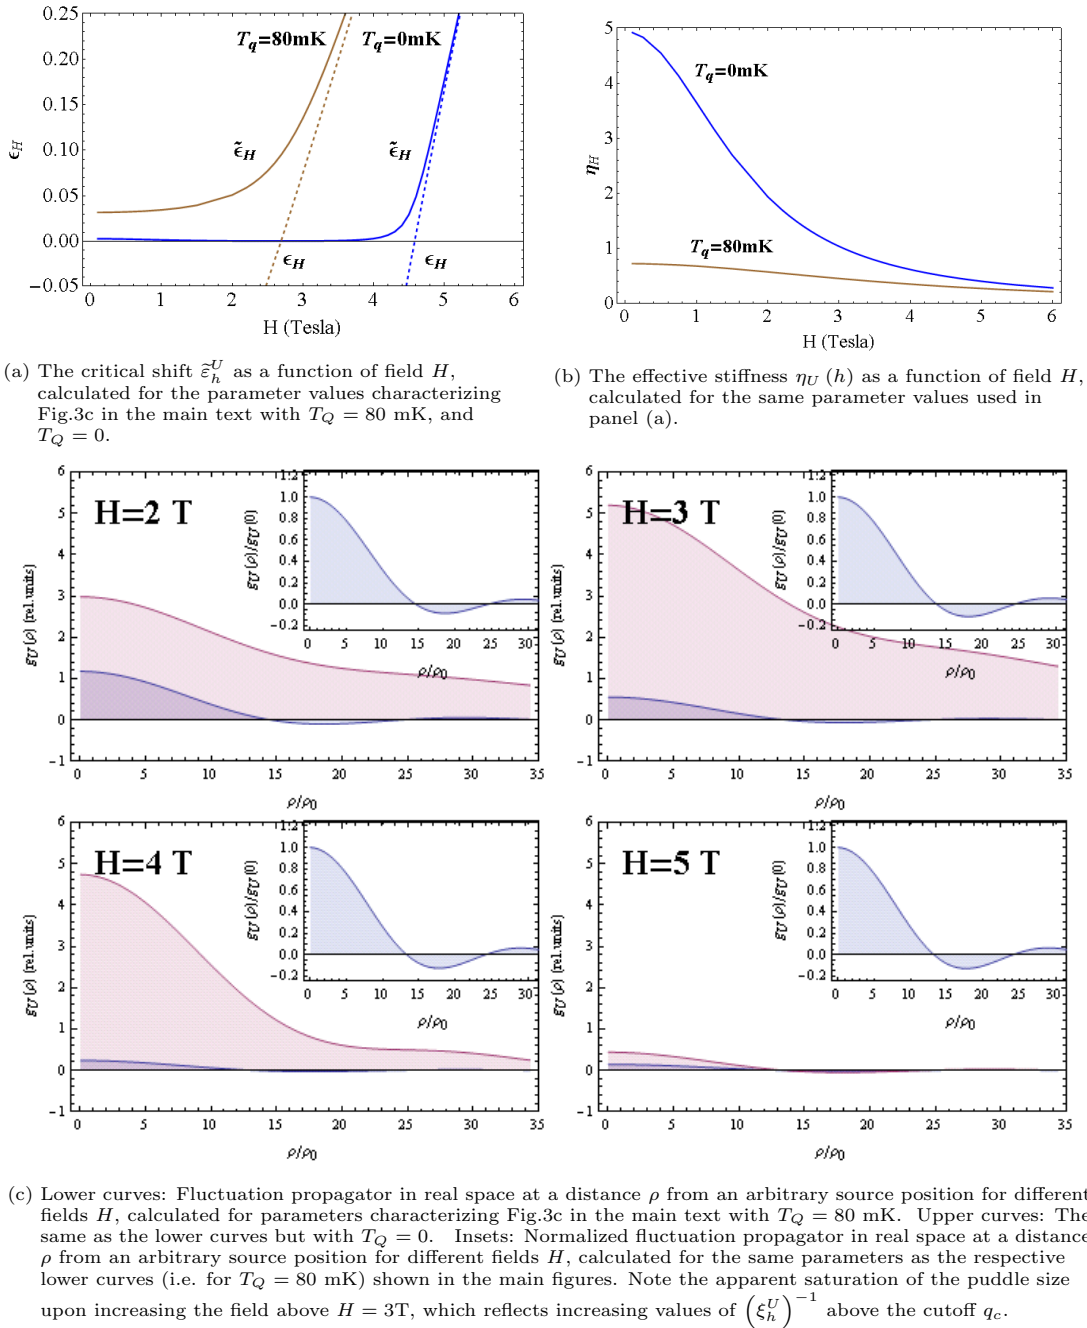

FIG. 3

$$n_s^Q \equiv (g_U(0))_{T \rightarrow 0} = \frac{2}{\pi \eta_Q(h)} \left( \frac{\varepsilon_{SO}}{E_F} \right) n_{2D} \ln \left[ 1 + (q_c \xi_h^Q)^2 \right]$$

The physical picture emerging from the analysis above is the following: Upon increasing the magnetic field towards the sheet-resistance peak region the 2D superconducting fluctuations system breaks into mesoscopic puddles of localized Cooper-pair, which consume much of the unpaired mobile electrons dominating the normal state conductivity. The localization arises from enhancement of the energy gap,  $\tilde{\epsilon}_h$ , of the fluctuations spectrum and suppression of the their effective stiffness coefficient,  $\hbar D \eta(h)$ , occurring upon increasing magnetic field. In parallel with this localization process upon increasing field, the paraconductivity,  $\sigma_{AL}$  decreases more sharply than  $-\delta \sigma_{DOS}$ , so that at the point of their crossing (see Fig.(4)) one observes the onset of the insulating state.

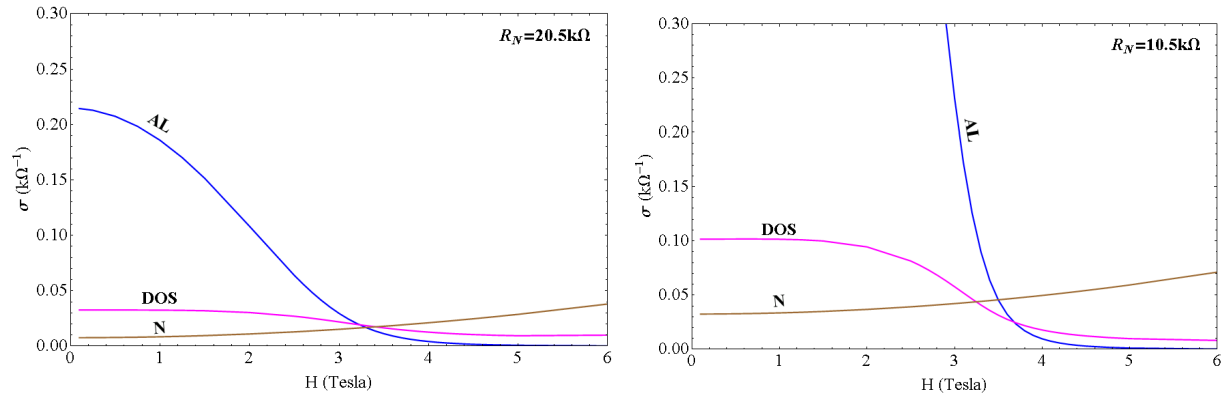

FIG. 4 Left panel:  $\sigma_{AL}$ ,  $-\delta\sigma_{DOS}$ , and  $\sigma_n$  contributing to the sheet conductance as functions of field  $H$ , calculated with the parameters used in Fig.3c of the main text, i.e. for  $R_N = 20.5\text{k}\Omega$ , ( $\alpha = 0.3$ ). Right panel: The same as the left panel calculated with the parameters used in Fig.3b of the main text, i.e. for  $R_N = 10.5\text{k}\Omega$  ( $\alpha = 0.11$ ). Note the crossing of  $\sigma_{AL}$  and  $-\delta\sigma_{DOS}$  at the onset of the respective MSR peak for each  $R_N$  value.

However, in this fields-range, where the AL conductivity is negligible, and quantum fluctuations diminish the localized Cooper-pairs puddles, the reinforced conductivity of the unpaired mobile electrons considerably smears the sheet resistance peak developed at very low temperatures. On the other hand, in the low-fields region, where the AL conductivity is dominant, finite resistance is generated (even at zero temperature) by quantum fluctuations due to enhanced localization of Cooper-pairs in SC puddles.

#### Sheet resistance of strongly interacting fluctuations

The self-consistent interaction parameter  $\alpha(R_N)$  that controls the SIT in our model depends on the Fermi energy of the high mobility carriers through the interpolation DOS function  $\nu(E_F)$  (see Eq.55). Upon increasing  $R_N$  (decreasing  $E_F$ ) from  $10.5\text{k}\Omega$  (7.2 meV) towards  $20.5\text{k}\Omega$  (6.5 meV), across the mixed-bands Lifshitz transition region,  $\alpha(R_N)$  increases by a factor of about 3 (see Table I). The corresponding increase of the critical shift (energy gap) parameter  $\varepsilon_h^U$  yields a large drop in  $\sigma_{AL}^U d$  and a significantly smaller reduction in  $-\delta\sigma_{DOS}^U d$ , which is balanced by a corresponding decrease in  $\sigma_n d$ , as clearly seen in Fig.(4) upon moving from the right to the left panel.

Consequently, in the low fields region, where the AL conductivity is dominant, its strong suppression upon increasing  $R_N$  from  $10.5\text{k}\Omega$  to  $20.5\text{k}\Omega$  leads to the large enhancement of the quantum tunneling-induced sheet resistance seen in Fig.3c of the main text at  $T = 30$  mK, as compared to that seen in Fig.3b.

In the high-fields region, near the crossing of  $\sigma_{AL}^U d$  with  $-\delta\sigma_{DOS}^U d$ , the suppression of all three components of the sheet conductance upon increasing  $R_N$  from  $10.5\text{k}\Omega$  to  $20.5\text{k}\Omega$  yields the significant enhancement of the sheet resistance peak seen in Fig.3c of the main text at  $T = 30$  mK, as compared to that seen in Fig.3b.

- 
- [1] A. A. Abrikosov and L.P. Gorkov, Zh. Exp. Teor. Fiz. 42, 1088 (1962) [Sov. Phys.-JETP **15**, 752 (1962)]
  - [2] R. A. Klemm, A. Luther and M.R. Beasley, "Theory of the upper critical field in layered superconductors", Phys. Rev. B **12**, 877 (1975).
  - [3] A. D. Caviglia, M. Gabay, S. Gariglio, N. Reyren, C. Cancellieri, and J.-M. Triscone, "Tunable Rashba Spin-Orbit Interaction at Oxide Interfaces", Phys. Rev. Lett. **104**, 126803 (2010).
  - [4] N. R. Werthamer, E. Helfand, and P. C. Hohenberg, "Temperature and Purity Dependence of the Superconducting Critical Field  $H_{c2}$ . III. Electron Spin and Spin-Orbit Effects", Phys. Rev. **147**, 295 (1966).
  - [5] K. Maki, "Effect of Pauli Paramagnetism on Magnetic Properties of High-Field Superconductors", Phys. Rev. **148**, 362 (1966).
  - [6] P. Fulde and K. Maki, "Fluctuations in High Field Superconductors", Z. Physik **238**, 233–248 (1970).
  - [7] M. Diez, A. M. R. V. L. Monteiro, G. Mattoni, E. Cobanera, T. Hyart, E. Mulazimoglu, N. Bovenzi, C.W. J. Beenakker, and A. D. Caviglia, "Giant Negative Magnetoresistance Driven by Spin-Orbit Coupling at the  $\text{LaAlO}_3/\text{SrTiO}_3$  Interface", Phys. Rev. Lett. **115**, 016803 (2015).
  - [8] Udit Khanna, P. K. Rout, Michael Mograbi, Gal Tuvia, Inge Leermakers, Uli Zeitler, Yoram Dagan, and Moshe Goldstein, "Symmetry and Correlation Effects on Band Structure Explain the Anomalous Transport Properties of (111)  $\text{LaAlO}_3/\text{SrTiO}_3$ ", Phys. Rev. Lett. **123**, 036805 (2019).
  - [9] S. Ullah and A.T. Dorsey, "Critical Fluctuations in High-Temperature Superconductors and the Ettingshausen Effect", Phys. Rev. Lett. **65**, 2066 (1990).



- [10] H. Schmidt, Zeitschrift fur Physik **216**, 336-345 (1968).
- [11] A. Larkin and A. Varlamov, "Theory of fluctuations in superconductors", Oxford University Press 2005.
- [12] M. Mograbi, E. Maniv, P. K. Rout, D. Graf, J. -H Park and Y. Dagan, "Vortex excitations in the Insulating State of an Oxide Interface", Phys. Rev. B **99**, 094507 (2019).
- [13] P. Rout, E. Maniv and Y. Dagan, "Link between the Superconducting Dome and Spin-Orbit Interaction in the (111) LaAlO<sub>3</sub>/SrTiO<sub>3</sub> Interface", Phys. Rev. Lett. **119**, 237002 (2017).
- [14] P. K. Rout, I. Agireen, E. Maniv, M. Goldstein, and Y. Dagan, "Six-fold crystalline anisotropic magnetoresistance in the (111) LaAlO<sub>3</sub>/SrTiO<sub>3</sub> oxide interface", Phys. Rev. B **95**, 241107(R) (2017).
- [15] K.Yu. Arutyunov, D.S. Golubev, A.D. Zaikin, "Superconductivity in one dimension", Phys. Rep. **464**, 1-70 (2008).
